# Supplementary material for: Competing magnetic orders and multipolar Weyl fermions in 227 pyrochlore iridates
Source: arXiv:2012.10442 ancillary file (2021-06-25)
Supplement: Supplementary file 1 [file Supplementary_V7.pdf]

# Supplementary Material: Competing magnetic orders and multipolar Weyl fermions in 227 pyrochlore iridates

Konstantinos Ladovrechis,<sup>1</sup> Tobias Meng,<sup>1</sup> and Bitan Roy<sup>2,3</sup>

<sup>1</sup>*Institute of Theoretical Physics, Technische Universität Dresden, 01062 Dresden, Germany*

<sup>2</sup>*Max-Planck-Institut für Physik komplexer Systeme, Nöthnitzer Str. 38, 01187 Dresden, Germany*

<sup>3</sup>*Department of Physics, Lehigh University, Bethlehem, Pennsylvania 18015, USA*

(Dated: December 18, 2020)

The Supplemental Materials contain (a) details of the Luttinger model [Sec. S1], (b) projection of various electronic magnetic orders on the pyrochlore lattice onto the low-energy Luttinger subspace [Sec. S2], (c) Fierz relations among interactions in various magnetic channels [Sec. S3], (d) derivation of the microscopic interacting Hamiltonian with on-site Hubbard ( $U$ ) and nearest-neighbor ferromagnetic ( $J$ ) interactions [Sec. S4], and (e) key steps for the mean field analysis [Sec. S5].

## S1. LUTTINGER MODEL

The Luttinger model from Eq. (1) of the main text can be rewritten as

$$\hat{H}(\mathbf{k}) = \frac{\hbar^2 k^2}{2m_0} \Gamma_0 - \frac{\hbar^2}{2m_1} \sum_{j=1}^3 \hat{d}_j(\hat{\mathbf{k}}) \Gamma_j - \frac{\hbar^2}{2m_2} \sum_{j=4}^5 \hat{d}_j(\hat{\mathbf{k}}) \Gamma_j, \quad (\text{S1})$$

where

$$\begin{aligned} \hat{d}_1(\hat{\mathbf{k}}) &= \frac{i[Y_2^1 + Y_2^{-1}]}{\sqrt{2}} = \frac{\sqrt{3}}{2} \sin 2\theta \sin \phi = \sqrt{3} \hat{k}_y \hat{k}_z, \quad \hat{d}_2(\hat{\mathbf{k}}) = \frac{[Y_2^{-1} + Y_2^1]}{\sqrt{2}} = \frac{\sqrt{3}}{2} \sin 2\theta \cos \phi = \sqrt{3} \hat{k}_x \hat{k}_z, \\ \hat{d}_3(\hat{\mathbf{k}}) &= \frac{i[Y_2^{-2} + Y_2^{-2}]}{\sqrt{2}} = \frac{\sqrt{3}}{2} \sin^2 \theta \sin 2\phi = \sqrt{3} \hat{k}_y \hat{k}_x, \quad \hat{d}_4(\hat{\mathbf{k}}) = \frac{[Y_2^{-2} + Y_2^2]}{\sqrt{2}} = \frac{\sqrt{3}}{2} \sin^2 \theta \cos 2\phi = \frac{\sqrt{3}}{2} [\hat{k}_x^2 - \hat{k}_y^2], \\ \hat{d}_5(\hat{\mathbf{k}}) &= Y_2^0 = \frac{1}{2} (3 \cos^2 \theta - 1) = \frac{1}{2} [2\hat{k}_z^2 - \hat{k}_x^2 - \hat{k}_y^2], \end{aligned} \quad (\text{S2})$$

and mutually anticommuting four-component Hermitian  $\Gamma$  matrices are

$$\Gamma_1 = \kappa_3 \sigma_2, \Gamma_2 = \kappa_3 \sigma_1, \Gamma_3 = \kappa_2 \sigma_0, \Gamma_4 = \kappa_1 \sigma_0, \Gamma_5 = \kappa_3 \sigma_3. \quad (\text{S3})$$

Two sets of Pauli matrices  $\{\kappa_\mu\}$  and  $\{\sigma_\mu\}$  with  $\mu = 0, \dots, 3$  operate on the sign and magnitude of the spin projection  $m_s = \pm 3/2, \pm 1/2$ , respectively. Here  $\Gamma_0 = \kappa_0 \sigma_0$  is a four-dimensional identity matrix. The Luttinger spinor is defined

$$\Psi^\dagger \equiv \Psi_{\mathbf{k}}^\dagger = (c_{\mathbf{k}, +\frac{3}{2}}^\dagger, c_{\mathbf{k}, +\frac{1}{2}}^\dagger, c_{\mathbf{k}, -\frac{1}{2}}^\dagger, c_{\mathbf{k}, -\frac{3}{2}}^\dagger) \quad (\text{S4})$$

where  $c_{\mathbf{k}, m_s}^\dagger$  is the fermion creation operator with momentum  $\mathbf{k}$  and spin projection  $m_s = \pm 3/2, \pm 1/2$ .

## S2. CONNECTING MICROSCOPIC SPIN PATTERNS TO THE LUTTINGER HAMILTONIAN

As explained in the main text, pyrochlore iridates can at low energies be modeled by a Luttinger Hamiltonian. This Hamiltonian can be obtained from a more microscopic non-interacting model containing eight bands via projection onto the relevant low-energy bands. The details thereof are explained in the Appendix A of Ref. [1]. The eight band-model describes four sites per unit cell, each of which harbors a spin-1/2 fermion. We can thus write the  $(8 \times 8)$ -model in the basis defined by the spinor

$$\psi^\dagger = (\hat{c}_{1,\uparrow,\mathbf{k}}^\dagger, \hat{c}_{1,\downarrow,\mathbf{k}}^\dagger, \hat{c}_{2,\uparrow,\mathbf{k}}^\dagger, \hat{c}_{2,\downarrow,\mathbf{k}}^\dagger, \hat{c}_{3,\uparrow,\mathbf{k}}^\dagger, \hat{c}_{3,\downarrow,\mathbf{k}}^\dagger, \hat{c}_{4,\uparrow,\mathbf{k}}^\dagger, \hat{c}_{4,\downarrow,\mathbf{k}}^\dagger) \quad (\text{S5})$$

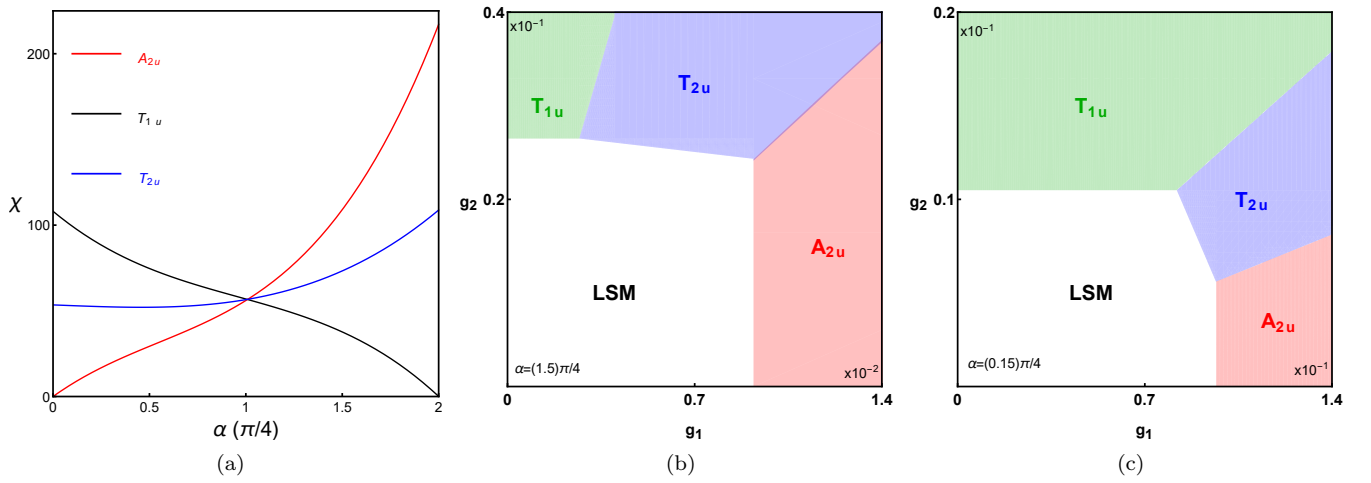

Figure S1: (a) Bare dimensionless susceptibilities ( $\chi$ ) for the  $A_{2u}$  (red),  $T_{1u}$  (black) and  $T_{2u}$  (blue) orders as a function of the mass anisotropy parameter  $\alpha$  (measured in units of  $\pi/4$ ) of the Luttinger model [see Eq. (1) and caption of Fig. 2 of the main text]. The dimensionless susceptibility is obtained by taking  $\chi[\Lambda(2m_p)^{3/2}/(32\pi^3)]^{-1} \rightarrow \chi$ . Only in the isotropic system ( $\alpha = \pi/4$ ) susceptibilities for three orders are degenerate, where the system enjoys a full  $SO(3)$  rotational symmetry. Here  $\alpha = \tan^{-1}(m_1/m_2)$  is the mass anisotropy parameter with  $0 \leq \alpha \leq \pi/2$ , and  $m_p = m_1 m_2 / (m_1 + m_2)$  [see Eq. (S1)]. The inverse of the bare susceptibility yields the critical coupling for the nucleation of the corresponding order. We use this information to construct two cuts of the phase diagram of a model with  $g_3^{(3)} = 0$  in Eq. (S26) in extreme anisotropic Luttinger system with (b)  $\alpha = 1.5(\pi/4)$  and (c)  $\alpha = 0.15(\pi/4)$ . Even though the bare interaction in the  $T_{2u}$  channel is zero, and effective interaction in this channel develops due to its competing nature with the  $A_{2u}$  (supported by  $g_1$ ) and  $T_{1u}$  (supported by  $g_2$ ) orders, manifested by the Fierz identity (see Sec. S3). Note that the phase boundaries between the ordered states is only for the purpose of clarity, as the computation of  $\chi$  only provides the phase boundaries between the disordered Luttinger semimetal and the ordered states.

where  $c_{i,s,\mathbf{k}}^\dagger$  creates a fermion at site  $i = 1, 2, 3, 4$  with spin  $s = \uparrow, \downarrow$  and momentum  $\mathbf{k}$ . Using the vector of Pauli matrices  $\boldsymbol{\sigma} = (\sigma_x, \sigma_y, \sigma_z)^T$ , the Fourier transforms of the fermionic spin operators in  $\hat{\mathbf{r}}$ -direction are then given by

$$\begin{aligned} \hat{S}_{1,\hat{\mathbf{r}}} &= \frac{\hbar}{2} \hat{\psi}^\dagger \text{Diag.}(\boldsymbol{\sigma} \cdot \hat{\mathbf{r}}, 0, 0, 0) \hat{\psi} \quad \text{and} \quad \hat{S}_{2,\hat{\mathbf{r}}} = \frac{\hbar}{2} \hat{\psi}^\dagger \text{Diag.}(0, \boldsymbol{\sigma} \cdot \hat{\mathbf{r}}, 0, 0) \hat{\psi} \\ \text{and} \quad \hat{S}_{3,\hat{\mathbf{r}}} &= \frac{\hbar}{2} \hat{\psi}^\dagger \text{Diag.}(0, 0, \boldsymbol{\sigma} \cdot \hat{\mathbf{r}}, 0) \hat{\psi} \quad \text{and} \quad \hat{S}_{4,\hat{\mathbf{r}}} = \frac{\hbar}{2} \hat{\psi}^\dagger \text{Diag.}(0, 0, 0, \boldsymbol{\sigma} \cdot \hat{\mathbf{r}}) \hat{\psi}. \end{aligned} \quad (\text{S6})$$

The projection of a fermionic bilinear operator  $\hat{\psi}^\dagger \mathcal{O}_{8 \times 8} \hat{\psi}$  represented by an  $(8 \times 8)$ -matrix  $\mathcal{O}_{8 \times 8}$  to the low-energy sector is achieved via

$$\mathcal{O}_{4 \times 4} = P_L \mathcal{O}_{8 \times 8} P_R, \quad (\text{S7})$$

where

$$P_L = \begin{pmatrix} -\frac{1/2 + i/2}{\sqrt{2}} & 0 & \frac{1/2 + i/2}{\sqrt{2}} & 0 & -\frac{1/2 - i/2}{\sqrt{2}} & 0 & \frac{1/2 - i/2}{\sqrt{2}} & 0 \\ \frac{1}{\sqrt{6}} & -\frac{1/2 + i/2}{\sqrt{6}} & \frac{1}{\sqrt{6}} & \frac{1/2 + i/2}{\sqrt{6}} & -\frac{1}{\sqrt{6}} & -\frac{1/2 - i/2}{\sqrt{6}} & \frac{1}{\sqrt{6}} & \frac{1/2 - i/2}{\sqrt{6}} \\ \frac{1/2 - i/2}{\sqrt{6}} & \frac{1}{\sqrt{6}} & -\frac{1/2 - i/2}{\sqrt{6}} & \frac{1}{\sqrt{6}} & \frac{1/2 + i/2}{\sqrt{6}} & \frac{1}{\sqrt{6}} & -\frac{1/2 + i/2}{\sqrt{6}} & \frac{1}{\sqrt{6}} \\ 0 & \frac{1/2 - i/2}{\sqrt{2}} & 0 & -\frac{1/2 - i/2}{\sqrt{2}} & 0 & \frac{1/2 + i/2}{\sqrt{2}} & 0 & -\frac{1/2 + i/2}{\sqrt{2}} \end{pmatrix} \quad (\text{S8})$$

and  $P_R = P_L^\dagger$  such that  $P_L P_R = \mathbb{1}_{4 \times 4}$ . Once projected down, the corresponding operator in the  $(4 \times 4)$ -model can be represented in terms of  $\Gamma$ -matrices. Because different  $\Gamma$ -matrices anticommute, they all square to  $\mathbb{1}_{4 \times 4}$ , and their traces vanish, the coefficient multiplying  $\Gamma_i$  in the representation of an operator  $\mathcal{O}_{4 \times 4}$  is  $(1/4) \text{tr}\{\Gamma_i \mathcal{O}_{4 \times 4}\}$ . Applying

this general procedure to the spin operators, we for example find that the  $(4 \times 4)$ -representation of the spin- $x$  density at site  $i = 1$  is given by

$$\begin{aligned} \hat{S}_1^x = & -\frac{1}{4\sqrt{3}} \left( \hat{\Psi}^\dagger \Gamma_{45} \hat{\Psi} \right) - \frac{1}{12} \left[ \left( \hat{\Psi}^\dagger \Gamma_{12} \hat{\Psi} \right) + \left( \hat{\Psi}^\dagger \Gamma_{13} \hat{\Psi} \right) + \left( \hat{\Psi}^\dagger \Gamma_{23} \hat{\Psi} \right) - \left( \hat{\Psi}^\dagger \Gamma_{14} \hat{\Psi} \right) - 2 \left( \hat{\Psi}^\dagger \Gamma_{24} \hat{\Psi} \right) - \left( \hat{\Psi}^\dagger \Gamma_{34} \hat{\Psi} \right) \right] \\ & + \frac{1}{4\sqrt{3}} \left[ - \left( \hat{\Psi}^\dagger \Gamma_{35} \hat{\Psi} \right) + \left( \hat{\Psi}^\dagger \Gamma_{15} \hat{\Psi} \right) \right]. \end{aligned} \quad (\text{S9})$$

Similarly, the projection of the all-in-all-out (AIAO) order leads to  $\Gamma_{45}$  [see Eq. (3) of the main text], while the spin ice orders project to  $\Gamma_j \Gamma_{45}$  with  $j = 1, 2, 3$  [see Eq. (4) of the main text] within the Luttinger subspace.

Instead of projecting down, one can also unproject operators by reverting the projection procedure step by step and representing the additional matrix elements generated in that process by generic entries. In many cases, the final form of the unprojected operators can be further restricted, e.g., by demanding that they describe a spin pattern and are thus block-diagonal. In doing so, it is important to recall that any projection, also the one defined in Eq. (S7), leads to a loss of information. Numerous operators in the  $(8 \times 8)$ -model consequently project to the same  $(4 \times 4)$ -operator, and vice versa. We find that the family of block-diagonal  $(8 \times 8)$ -operators (i.e. operators that can in principle describe spin ordering patterns in the  $(8 \times 8)$ -model) projecting to the same  $(4 \times 4)$ -operator can be parametrized by two parameters  $\alpha$  and  $\beta$  as  $\mathcal{O}_{8 \times 8}(\alpha, \beta) = \mathcal{O}_{8 \times 8}^{(0)} + M(\alpha, \beta)$ , where  $\mathcal{O}_{8 \times 8}^{(0)}$  is one representative of the family, and where

$$\begin{aligned} M(\alpha, \beta) = & \text{Diag.} [\alpha(\sigma_x + \sigma_y) + \beta(\sigma_y + \sigma_z), -\alpha(\sigma_x + \sigma_y) + \beta(-\sigma_y + \sigma_z), \\ & \alpha(\sigma_x - \sigma_y) - \beta(\sigma_y + \sigma_z), \alpha(-\sigma_x + \sigma_y) + \beta(\sigma_y - \sigma_z)] \end{aligned} \quad (\text{S10})$$

projects to zero,  $P_L M(\alpha, \beta) P_R = 0$ . With this procedure, we find that one set of representatives of the  $\hat{T}_{2u}$  orders in the  $(8 \times 8)$ -model is

$$O_{T_{2u}^{(1)}} = \frac{\sqrt{3}}{2} \text{Diag.} [\sigma_z + \sigma_y, -\sigma_z + \sigma_y, -\sigma_z - \sigma_y, \sigma_z - \sigma_y], \quad (\text{S11})$$

$$O_{T_{2u}^{(2)}} = \frac{\sqrt{3}}{2} \text{Diag.} [\sigma_z - \sigma_x, -\sigma_z - \sigma_x, -\sigma_z + \sigma_x, -\sigma_z + \sigma_x], \quad (\text{S12})$$

$$O_{T_{2u}^{(3)}} = \frac{\sqrt{3}}{2} \text{Diag.} [-\sigma_x - \sigma_y, \sigma_x + \sigma_y, \sigma_x - \sigma_y, -\sigma_x + \sigma_y]. \quad (\text{S13})$$

The corresponding arrangements of electronic spin at four sites of the Ir tetrahedron are shown in Fig. 1 (lower panel) of the main text. Respectively  $O_{T_{2u}^{(1)}}$ ,  $O_{T_{2u}^{(2)}}$  and  $O_{T_{2u}^{(3)}}$  when projected onto the low-energy Luttinger subspace, their coupling with effective spin-3/2 fermions read  $\hat{T}_{2u}^{(1)}$ ,  $\hat{T}_{2u}^{(2)}$  and  $\hat{T}_{2u}^{(3)}$  [see Eq. (5) of the main text]. When  $\alpha \neq 0$  or  $\beta \neq 0$ , the matrices  $O_{T_{2u}^{(i)}} + M(\alpha, \beta)$  can easily be seen to give rise to various rescaled and rotated versions of other spin microscopic patterns.

### S3. INTERACTIONS AND FIERZ IDENTITIES IN PYROCHLORE IRIDATES

A generic local density-density interaction model for spin-3/2 fermions contains 136 quartic terms, but the number of non-zero interaction constants is usually strongly restrained by symmetries, and reduces to only *six* [1, 2]. In addition, different representations of interactions among spin-3/2 fermions can be transformed into each other by virtue of Fierz identities [4], which further reduces the number of independent interactions. Fierz identities are essentially based on reorderings of fermionic operators, and generalize the identity  $(c_\alpha^\dagger c_\alpha)(c_\beta^\dagger c_\beta) + (c_\alpha^\dagger c_\beta)(c_\beta^\dagger c_\alpha) = 0$  that holds for two different fermionic operators  $c_\alpha$  and  $c_\beta$ . Following Ref. [3], one can show that there are three Fierz identities for our

problem, which take the form [2]

$$2(\hat{\Psi}^\dagger \Gamma_{45} \hat{\Psi})^2 + (\hat{\Psi}^\dagger \Gamma_0 \hat{\Psi})^2 + \sum_{j=1}^3 (\hat{\Psi}^\dagger \Gamma_j \hat{\Psi})^2 - \sum_{j=4}^5 (\hat{\Psi}^\dagger \Gamma_j \hat{\Psi})^2 = 0, \quad (\text{S14})$$

$$2 \sum_{j=1}^3 (\hat{\Psi}^\dagger \Gamma_j \Gamma_{45} \hat{\Psi})^2 + 3(\hat{\Psi}^\dagger \Gamma_0 \hat{\Psi})^2 - \sum_{j=1}^3 (\hat{\Psi}^\dagger \Gamma_j \hat{\Psi})^2 + 3 \sum_{j=4}^5 (\hat{\Psi}^\dagger \Gamma_j \hat{\Psi})^2 = 0, \quad (\text{S15})$$

$$\sum_{j,k=1}^3 (\hat{\Psi}^\dagger \Gamma_j \Gamma_k \hat{\Psi})^2 + 3(\hat{\Psi}^\dagger \Gamma_0 \hat{\Psi})^2 + \sum_{j=1}^3 (\hat{\Psi}^\dagger \Gamma_j \hat{\Psi})^2 = 0. \quad (\text{S16})$$

While Fierz relations are exact operator identities, mean field decouplings of Fierz-equivalent representations of the same physical interaction neglect fluctuations in different channels. As a result, mean field theory in systems with Fierz identities is known to have a certain degree of ambiguity [5], which nonetheless is a typical shortcoming of any mean field analysis in systems with competing phases. The derivation of a detailed phase diagram therefore requires more involved techniques, such as unbiased renormalization group approaches. General trends, however, can often be inferred from mean field analysis, at least at the qualitative level.

Here, we use Fierz transformations as a resource to derive an estimate for the overall topology of the phase diagram in pyrochlore iridates. Our starting point is a phenomenological minimal interaction model that builds on the experimental observation of the dominant AIAO order and spin ice order in pyrochlore iridates. These two orders can be derived from a mean field analysis of the following phenomenological interacting Hamiltonian

$$\hat{H}_{\text{phen. int.}} = g_1 (\hat{\Psi}^\dagger \Gamma_{45} \hat{\Psi})^2 + g_2 \sum_{j=1}^3 (\hat{\Psi}^\dagger \Gamma_j \Gamma_{45} \hat{\Psi})^2. \quad (\text{S17})$$

In this notation  $g_j > 0$  corresponds to repulsive interaction. Otherwise, repulsive  $g_1$  and  $g_2$  interactions are conducive for the AIAO and spin-ice orders. Using the above Fierz relations, this Hamiltonian can be rewritten as

$$\hat{H}_{\text{phen. int.}} = g_3 \sum_{j=1}^3 (\hat{\Psi}^\dagger \Gamma_j \hat{\Psi})^2 + g_4 \sum_{j=4}^5 (\hat{\Psi}^\dagger \Gamma_j \hat{\Psi})^2 + g_5 \sum_{j=1}^3 \sum_{k=4}^5 (\hat{\Psi}^\dagger \Gamma_{jk} \hat{\Psi})^2 \quad (\text{S18})$$

with the new coupling constants

$$g_3 \equiv \frac{1}{3} (-g_1 + 3g_2), \quad g_4 \equiv \frac{1}{2} (g_1 - 3g_2), \quad g_5 \equiv \frac{1}{6} (g_1 + 3g_2). \quad (\text{S19})$$

The terms with coefficients  $g_3$  and  $g_4$  correspond to effective interactions in the  $T_{2g}$  and  $E_g$  nematic channels, respectively, whereas the last term with coefficient  $g_5$  describes tensorial magnetic interactions (including the  $T_{2u}$  channel). Therefore, even in a model that is most favorable to the formation of AIAO and spin ice orders, the  $T_{2u}$  order can in principle be nucleated, specifically when the interaction couplings in these two channels are comparably strong. To obtain an estimate for the relative positions of the phases we are interested in, we proceed by focusing on the AIAO, spin ice and  $T_{2u}^{(3)}$  orders. Comparing the Stoner criteria for these different orders given the interaction constants  $g_1$ ,  $g_2$ , and  $g_5 = (g_1 + 3g_2)/6$ , the present analysis places the  $T_{2u}$  order as an intermediate phase between AIAO or  $A_{2u}$  and spin ice or  $T_{1u}$  orders, as shown in Fig. S1. More detail on the mean field analysis is discussed in Sec. S5. The tendency towards the formation of such an intermediate phase is further boosted when the competition between different order parameters is taken into account. Consult the discussion on the selection algebra among competing magnetic phases and inset of Fig. 2 (inset) in the main text.

#### S4. MICROSCOPIC U-J MODEL FOR LUTTINGER FERMIONS

The interacting Hamiltonian in the presence of on-site Hubbard ( $U$ ) and nearest-neighbor ferromagnetic ( $J$ ) interaction among  $5d$  electrons of  $\text{Ir}^{4+}$  ions reads as [see also Eq. (9) of the main text]

$$H_{\text{mic}} = 3U \sum_{i=1}^4 \hat{S}_{i,111} \hat{S}_{i,111} + 3J \sum_{i \neq j=1}^4 \hat{S}_{i,111} \hat{S}_{j,111}, \quad (\text{S20})$$

where  $\hat{S}_{i,111}$  is the spin density operator at site  $i$  in the [111] direction defined in (S6) for  $\hat{\mathbf{r}} = (1, 1, 1)/\sqrt{3}$  and  $i = 1, 2, 3, 4$  correspond to four sites of an Ir tetrahedra. As the itinerant spins on pyrochlore lattice dominantly tend to lock in the body diagonal  $\langle 111 \rangle$  directions, here we for the sake of simplicity picked the magnetization along one of the body diagonal directions. In the basis of spinor (S5), the spin density operators along the [111] direction at the four sites of a single Ir tetrahedron read

$$\begin{aligned} \hat{S}_{1,111} &= \frac{\hbar}{2\sqrt{3}} \hat{\psi}^\dagger \text{Diag.}(\sigma_x + \sigma_y + \sigma_z, 0, 0, 0) \hat{\psi} \quad \text{and} \quad \hat{S}_{2,111} = \frac{\hbar}{2\sqrt{3}} \hat{\psi}^\dagger \text{Diag.}(0, \sigma_x + \sigma_y + \sigma_z, 0, 0) \hat{\psi} \\ \text{and} \quad \hat{S}_{3,111} &= \frac{\hbar}{2\sqrt{3}} \hat{\psi}^\dagger \text{Diag.}(0, 0, \sigma_x + \sigma_y + \sigma_z, 0) \hat{\psi} \quad \text{and} \quad \hat{S}_{4,111} = \frac{\hbar}{2\sqrt{3}} \hat{\psi}^\dagger \text{Diag.}(0, 0, 0, \sigma_x + \sigma_y + \sigma_z) \hat{\psi}. \end{aligned} \quad (\text{S21})$$

In the above expressions “0” stands for two-dimensional null matrix. After projecting the fermionic magnetization operators in the [111] direction to the four-dimensional low-energy Luttinger manifold of effective spin-3/2 fermions following the prescription from Ref. [1], we obtain

$$\begin{aligned} \hat{S}_{1,111}^{\text{Lutt}} &= \frac{1}{4\sqrt{3}} (\Psi^\dagger \Gamma_{45} \Psi) + \frac{1}{12} [(\Psi^\dagger \Gamma_{12} \Psi) + (\Psi^\dagger \Gamma_{13} \Psi) + (\Psi^\dagger \Gamma_{23} \Psi)] - \frac{1}{6} [2(\Psi^\dagger \Gamma_{14} \Psi) + (\Psi^\dagger \Gamma_{24} \Psi) - (\Psi^\dagger \Gamma_{34} \Psi)] \\ &+ \frac{1}{2\sqrt{3}} [(\Psi^\dagger \Gamma_{25} \Psi) + (\Psi^\dagger \Gamma_{35} \Psi)], \end{aligned} \quad (\text{S22})$$

$$\begin{aligned} \hat{S}_{2,111}^{\text{Lutt}} &= \frac{1}{4\sqrt{3}} (\Psi^\dagger \Gamma_{45} \Psi) + \frac{1}{12} [(\Psi^\dagger \Gamma_{12} \Psi) - (\Psi^\dagger \Gamma_{13} \Psi) - (\Psi^\dagger \Gamma_{23} \Psi)] - \frac{1}{6} [(\Psi^\dagger \Gamma_{14} \Psi) + 2(\Psi^\dagger \Gamma_{24} \Psi) - (\Psi^\dagger \Gamma_{34} \Psi)] \\ &- \frac{1}{2\sqrt{3}} [(\Psi^\dagger \Gamma_{15} \Psi) + (\Psi^\dagger \Gamma_{35} \Psi)], \end{aligned} \quad (\text{S23})$$

$$\begin{aligned} \hat{S}_{3,111}^{\text{Lutt}} &= \frac{1}{4\sqrt{3}} (\Psi^\dagger \Gamma_{45} \Psi) - \frac{1}{12} [(\Psi^\dagger \Gamma_{12} \Psi) + (\Psi^\dagger \Gamma_{13} \Psi) - (\Psi^\dagger \Gamma_{23} \Psi)] + \frac{1}{6} [(\Psi^\dagger \Gamma_{14} \Psi) + (\Psi^\dagger \Gamma_{24} \Psi) + 2(\Psi^\dagger \Gamma_{34} \Psi)] \\ &- \frac{1}{2\sqrt{3}} [(\Psi^\dagger \Gamma_{15} \Psi) - (\Psi^\dagger \Gamma_{25} \Psi)], \end{aligned} \quad (\text{S24})$$

$$\hat{S}_{4,111}^{\text{Lutt}} = -\frac{\sqrt{3}}{4} (\Psi^\dagger \Gamma_{45} \Psi) + \frac{1}{4} [(\Psi^\dagger \Gamma_{12} \Psi) - (\Psi^\dagger \Gamma_{13} \Psi) + (\Psi^\dagger \Gamma_{23} \Psi)]. \quad (\text{S25})$$

After obtaining the fermionic magnetization operator in the [111] direction in terms of the Luttinger spinor (S4), we obtain  $H_{\text{mic}}$  within the Luttinger manifold of spin-3/2 fermions, which when compared with the following effective model [see also Eq. (8)]

$$H_{\text{int}} = g_1 (\Psi^\dagger \hat{A}_{2u} \Psi)^2 + g_2 \sum_{j=1}^3 (\Psi^\dagger \hat{T}_{1u}^{(j)} \Psi)^2 + g_3^{(3)} (\Psi^\dagger \hat{T}_{2u}^{(3)} \Psi)^2, \quad (\text{S26})$$

one finds the following one-to-one correspondences among the coupling constants [see also Eq. (10) of the main text]

$$g_1 = \frac{U}{4} \left(1 - \frac{J}{2U}\right), \quad g_2 = \frac{U}{12} \left(1 + \frac{J}{6U}\right), \quad g_3^{(3)} = \frac{U}{6} \left(1 - \frac{J}{2U}\right). \quad (\text{S27})$$

We perform a mean-field analysis of this model to capture the competition between  $A_{2u}$ ,  $T_{1u}$  and  $T_{2u}$  magnetic orders, which are respectively favored by  $g_1$ ,  $g_2$  and  $g_3^{(3)}$ . Next we show the quintessential steps of this analysis.

## S5. MEAN-FIELD SUSCEPTIBILITY ANALYSIS AND PHASE DIAGRAM

We here restrict ourselves to the leading-order mean field analysis. We compute and compare bare susceptibilities for competing magnetic orders with zero external momentum and frequency to construct the phase diagrams, shown in Fig. 2 of the main text and in Fig. S1(b) and (c). The methodology is the following. A given quartic interaction  $g_M (\Psi^\dagger M \Psi)^2$ , where  $M$  is a Hermitian matrix in the mean field approximation is conducive for the nucleation of an ordered state, characterized by the order parameter  $\Psi^\dagger M \Psi$ . However, due to a vanishing density of states in Luttinger semimetal (namely,  $\rho(E) \sim \sqrt{E}$ ) such ordering sets in beyond a critical interaction coupling  $g_M^*$ , given by  $g_M^* = \chi_M^{-1}$ , where  $\chi_M$  is the bare mean field susceptibility for zero external momentum and frequency given by

$$\chi_M = - \int_{-\infty}^{\infty} \frac{d\omega}{2\pi} \int' \frac{d^3\mathbf{k}}{(2\pi)^3} \text{Tr} [M G(i\omega, \mathbf{k}) M G(i\omega, \mathbf{k})]. \quad (\text{S28})$$

Here  $G(i\omega, \mathbf{k}) = [i\omega - \hat{H}(\mathbf{k})]^{-1}$  is the fermionic Greens function,  $\omega$  is the fermionic Matsubara frequency, and the momentum integral is restricted up to an ultraviolet momentum cut off  $\Lambda$ , denoted by the prime ( $'$ ) symbol. For the sake of simplicity we neglect the particle hole anisotropy in the Luttinger Hamiltonian  $\hat{H}(\mathbf{k})$  [see Eq. (S1)]. Upon computing the mean field susceptibilities for the  $A_{2u}$ ,  $T_{1u}$  and  $T_{2u}$  magnetic orders [see Fig. S1(a)], we express their requisite critical coupling for nucleation in terms of  $U$  and  $J$  to construct the phase diagram shown in Fig. 2 of the main text following Eq. (S27). We follow the same procedure to construct the phase diagrams in the  $(g_1, g_2)$  plane, shown in Fig. S1(b) and (c). While constructing the two cuts of the phase diagrams in the  $(g_1, g_2)$  plane, we solely focus on the magnetic orders and neglect their competition with two nematic orders. Otherwise, the phase with minimal critical coupling corresponds to the ordered state for a given set of parameters.

- 
- [1] P. Goswami, B. Roy, and S. Das Sarma, Phys. Rev. B **95**, 085120 (2017).
  - [2] A. L. Szabó, R. Moessner, and B. Roy, arXiv:1811.12415
  - [3] I. F. Herbut, V. Juričić and B. Roy, Phys. Rev. B **79**, 085116 (2009).
  - [4] C. C. Nishi, Am. J. Phys. **73**, 1160 (2005).
  - [5] J. Jaeckel and C. Wetterich, Phys. Rev. D **68**, 025020 (2003).
